# Supplementary material for: An Efficient Deep Distribution Network for Bid Shading in First-Price Auctions
Source: arXiv:2107.06650 source file (2021-07-15)
Supplement: Supplementary file 1 [file 8.appendix.tex]

\begin{theorem}\label{thm:theorem1}
If $s(x)$ has less than three inflection points, then it must have one global maximum $b^{*}$ that can maximize the surplus \eqref{eq:expsurplus}
\end{theorem}
\begin{proof}
We prove it by its contradiction: if \eqref{eq:expsurplus} has more than 1 local/global maximum, then it must have at least three inflection points. \\
Due to the boundary condition of \eqref{eq:expsurplus}, in which s(0) = 0, s(V) = 0, and $s(x) > 0$, in order to have two local maximum, \eqref{eq:generalderv} must start from positive, become negative (at first local maximum), then positive (at local minimum), and finally negative (at second local/global maximum), which has at least three inflection points.
\end{proof}

\begin{theorem}\label{thm:theorem2}
If we assume that minimum bid to win follows a beta/gamma/normal/Log-normal distribution, there exists a unique solution $b^{*}$ that can maximize the surplus \eqref{eq:expsurplus}
\end{theorem}
\begin{proof}
for Gamma distribution with one mode, $$f(x) = \dfrac{\beta^{\alpha}}{\Gamma (\alpha)} x^{\alpha - 1}e^{-\beta x} $$
with $\alpha > 1$ and $\beta > 0$
$$f'(x) = \dfrac{\beta^{\alpha}}{\Gamma(\alpha)}x^{\alpha - 1}e^{-\beta x} \left( \frac{\alpha - 1}{x} - \beta \right) $$
From \eqref{eq:generalderv2}, 
\begin{eqnarray}
s''(x) & = & \dfrac{\beta^{\alpha}}{\Gamma(\alpha)}x^{\alpha - 1}e^{-\beta x}\left[\left(\frac{\alpha - 1}{x} - \beta\right)\left(V-x
\right) - 2\right] \nonumber \\ 
 & = & \dfrac{f(x)}{x}\left[\left(\alpha - 1 - \beta x\right)\left(V-x\right) - 2x\right] \nonumber \\ 
 & = & \dfrac{f(x)}{x} \left[ \beta x^2 - \left( \alpha + \beta V + 1 \right) x + \left( \alpha - 1 \right) V \right] \label{eq:gammaderv2}
\end{eqnarray}
Similarly, for beta distribution
\begin{align}
    s''(x) &= \frac{(V-x)}{B(\alpha,\beta)} \left[ (\alpha-1) x^{\alpha-2} (1-x)^{\beta-1} - (\beta-1) x^{\alpha-1} (1-x)^{\beta-2} \right] - 2 f(x) \ \nonumber \\
    &= \frac{(V-x)x^{\alpha-1}(1-x)^{\beta-1}}{B(\alpha,\beta)} \left[ (\alpha-1)\frac{1}{x} - (\beta-1)\frac{1}{1-x} \right] - 2f(x) \nonumber \\
    &= (V-x) f(x) \left[ (\alpha-1)\frac{1}{x} - (\beta-1)\frac{1}{1-x} \right] - 2f(x) \nonumber \\
    &= \frac{f(x)}{x (1-x)} \left[ (V-x)(\alpha-1)(1-x) - (V-x)(\beta-1)x - 2x(1-x) \right] \nonumber \\
    &= \frac{f(x)}{x (1-x)} [(\alpha+\beta) x^2 + (2V - \alpha V - \beta V - \alpha - 1)x + (\alpha V - V)] \label{eq:betaderv2}
\end{align}
We can see s(x) has at most 2 inflection points as its second derivative \eqref{eq:gammaderv2} and \eqref{eq:betaderv2} are second order functions, which complete the proof according to \ref{thm:theorem2}. \\

For Gaussian distribution, whose pdf is as follows
$$
f_{\text{Gaussian}}(x) = \frac{1}{\sigma \sqrt{2\pi}} \exp{\left(-\frac{(x-\mu)^2}{2\sigma^2}\right)}
$$
\begin{align}
    s''(x) &= f'_{\text{Gaussian}}(x)[v-x]-2f_{\text{Gaussian}}(x)  \nonumber \\
    & = f_{\text{Gaussian}}(x)(-\frac{x-\mu}{\sigma^2})(v-x)-2f_{\text{Gaussian}}(x) \nonumber \\
    & = f_{\text{Gaussian}}(x) \left( \frac{(\mu-x)(v-x)}{\sigma^2} -2 \right)
\label{eq:gaussian}
\end{align}
As can be seen that $f_{\text{Gaussian}}(x) > 0$, the second order polynomial has at most two solutions on $[0,v]$. \\

For log-normal distribution, with the following pdf 
$$
f_{\text{l-n}}(x) = \frac{1}{x\sigma \sqrt{2\pi}} \exp{\left(-\frac{(\ln(x)-\mu)^2}{2\sigma^2}\right)}
$$

\begin{align}
    s''(x) &= f'_{\text{l-n}}(x)[v-x]-2f_{\text{l-n}}(x)  \nonumber \\
    & = f_{\text{l-n}}(x)(-\frac{1}{x} -\frac{1}{x}\frac{\ln(x)-\mu}{\sigma^2})(v-x)-2f_{\text{l-n}}(x) \nonumber \\
    & = \frac{f_{\text{l-n}}(x)}{-x} \left( \frac{\sigma^2+\ln(x)-\mu}{\sigma^2}(v-x) +2x \right) \nonumber \\
    & = \frac{f_{\text{l-n}}(x)}{-x \sigma^2} \left( (\sigma^2+\ln(x)-\mu)(v-x) +2x\sigma^2 \right)
\label{eq:lognormal}
\end{align}
Let $$t(x) = (\sigma^2+\ln(x)-\mu)(v-x) +2x\sigma^2,$$
it can be shown that $$t''(x) = -\frac{v}{x^2} - \frac{1}{x} < 0 $$, is less than 0 on $[0, v]$. Thus, the function $t(x)$ is concave and has at most two roots.

\end{proof}
